# Supplementary material for: Interface-templated crystal growth in sodium dodecyl sulfate solutions with NaCl
Source: arXiv:2311.03544 source file (2023-11-10)
Supplement: Supplementary file 1 [file SI.pdf]

# Supplementary information: Interface-templated crystal growth in sodium dodecyl sulfate solutions with NaCl

Anna Kharlamova[1,2], François Boulogne[1], Philippe Fontaine[2], Stéphan Rouzière[1], Arnaud Hemmerle[2], Michel Goldmann[2,3], and Anniina Salonen[1,*]

[1]Université Paris-Saclay, CNRS, Laboratoire de Physique des Solides, 91405, Orsay, France.
[2]Synchrotron SOLEIL, L'Orme des Merisiers, Départementale 128, 91190, Saint-Aubin, France.
[3]Institut des NanoSciences de Paris, Sorbonne Université, 4 Place Jussieu, 75005 Paris, France.

[*]Corresponding author: anniina.salonen@universite-paris-saclay.fr

## 1 Movies

**Video 1:** Video of a Petri dish during the crystallization process from a sample with 0.6 mM SDS with 500 mM Nacl. A time-stamp indicates the time starting from as the solution is poured into the Petri dish.

**Video 2:** Video of a Petri dish during the crystallization process from a sample with 1.0 mM SDS with 500 mM Nacl. A time-stamp indicates the time starting from as the solution is poured into the Petri dish.

## 2 Krafft temperature

Figure S1 shows our measurements of the Krafft temperature of SDS with NaCl at four different surfactant concentrations. Raw data are presented in table S1.

## 3 WAXS measurements of bulk crystal structure

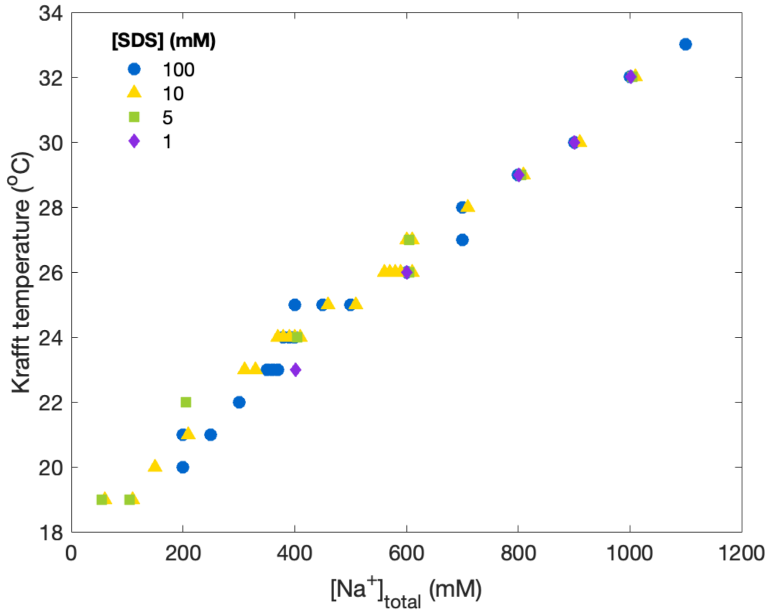


Figure S1: Krafft temperature as the function of the total concentration of $Na^+$ ions for four different concentrations of SDS.

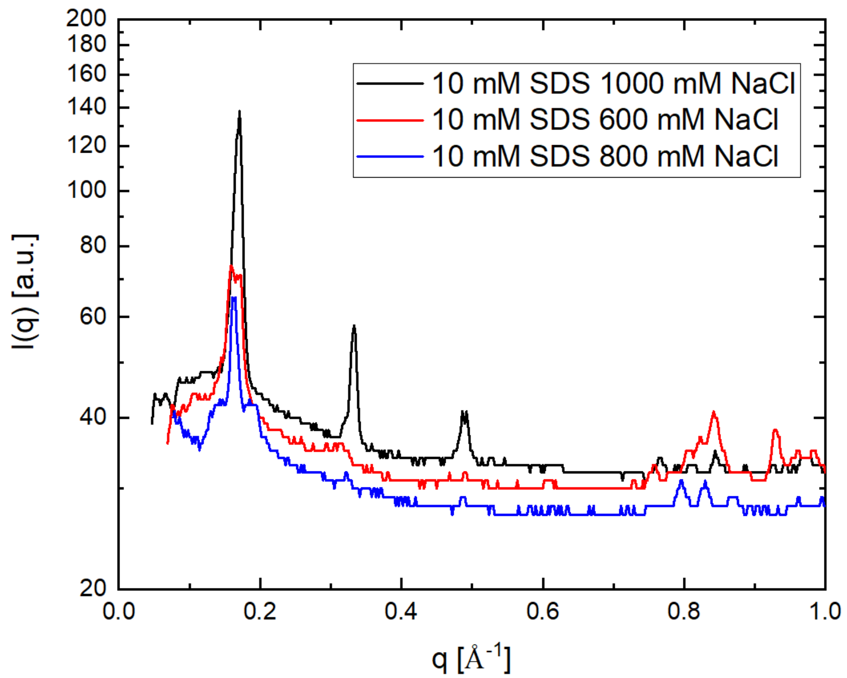


Figure S2: Scattered intensity as a function of the q-vector for SDS precipitated in 600, 800 or 1000 mM NaCl solutions. The SDS concentration used is 10 mM in all the samples.

(a)

| [SDS] (mM) | [NaCl] (mM) | $[Na^+]$ (mM) | $T_K$ (°C) |
|---|---|---|---|
| 1 | 400 | 401 | 23 |
| 1 | 600 | 601 | 26 |
| 1 | 800 | 801 | 29 |
| 1 | 900 | 901 | 30 |
| 1 | 1000 | 1001 | 32 |

(b)

| [SDS] (mM) | [NaCl] (mM) | $[Na^+]$ (mM) | $T_K$ (°C) |
|---|---|---|---|
| 5 | 50 | 55 | 19 |
| 5 | 100 | 105 | 19 |
| 5 | 200 | 205 | 22 |
| 5 | 400 | 405 | 24 |
| 5 | 600 | 605 | 26 |
| 5 | 600 | 605 | 27 |
| 5 | 800 | 805 | 29 |
| 5 | 1000 | 1005 | 32 |

(c)

| [SDS] (mM) | [NaCl] (mM) | $[Na^+]$ (mM) | $T_K$ (°C) |
|---|---|---|---|
| 10 | 50 | 60 | 19 |
| 10 | 100 | 110 | 19 |
| 10 | 140 | 150 | 20 |
| 10 | 200 | 210 | 21 |
| 10 | 300 | 310 | 23 |
| 10 | 320 | 330 | 23 |
| 10 | 360 | 370 | 24 |
| 10 | 370 | 380 | 24 |
| 10 | 380 | 390 | 24 |
| 10 | 390 | 400 | 24 |
| 10 | 400 | 410 | 24 |
| 10 | 450 | 460 | 25 |
| 10 | 500 | 510 | 25 |
| 10 | 550 | 560 | 26 |
| 10 | 560 | 570 | 26 |
| 10 | 570 | 580 | 26 |
| 10 | 580 | 590 | 26 |
| 10 | 590 | 600 | 27 |
| 10 | 600 | 610 | 26 |
| 10 | 600 | 610 | 27 |
| 10 | 700 | 710 | 28 |
| 10 | 800 | 810 | 29 |
| 10 | 900 | 910 | 30 |
| 10 | 1000 | 1010 | 32 |

(d)

| [SDS] (mM) | [NaCl] (mM) | $[Na^+]$ (mM) | $T_K$ (°C) |
|---|---|---|---|
| 100 | 100 | 200 | 21 |
| 100 | 100 | 200 | 20 |
| 100 | 150 | 250 | 21 |
| 100 | 200 | 300 | 22 |
| 100 | 250 | 350 | 23 |
| 100 | 260 | 360 | 23 |
| 100 | 270 | 370 | 23 |
| 100 | 280 | 380 | 24 |
| 100 | 290 | 390 | 24 |
| 100 | 300 | 400 | 25 |
| 100 | 300 | 400 | 24 |
| 100 | 350 | 450 | 25 |
| 100 | 400 | 500 | 25 |
| 100 | 500 | 600 | 26 |
| 100 | 600 | 700 | 27 |
| 100 | 600 | 700 | 28 |
| 100 | 700 | 800 | 29 |
| 100 | 800 | 900 | 30 |
| 100 | 900 | 1000 | 32 |
| 100 | 1000 | 1100 | 33 |

Table S1: Data used in figure S1 presented for (a) 1 mM, (b) 5 mM, (c) 10 mM, and (d) 100 mM SDS concentrations. $T_K$ is the Krafft temperature measured at ±1°C.
